# Supplementary material for: Price Cuts and the Information in Purchases
Source: arXiv:2509.01263 ancillary file (2026-11-29)
Supplement: Supplementary file 1 [file HerdingPrices_slides.pdf]

# Herding Prices:

## Social Learning and Dynamic Competition in Duopoly

Georgy Lukyanov    Arina Azova

# Plan

- ① Motivation & empirical flavor
- ② Model in two minutes
- ③ Learning: threshold rule, cascade bands, absorption
- ④ Static price competition: existence, dispersion, C.S.
- ⑤ Comparative statics & welfare
- ⑥ Extensions: Calvo resets, prominence, noisy reviews
- ⑦ Takeaways

# Motivation

- Consumers see *actions* (purchases) and prices; they do *not* see payoffs.
- Early purchases tilt subsequent choices  $\Rightarrow$  belief feedback  $\Rightarrow$  cascades.
- Firms best-respond with prices; prices in turn shape informativeness (search/checking).
- Questions:
  - When do we herd? How often are herds *wrong*? How fast do we get there?
  - Do symmetric firms price in mixed strategies? What drives dispersion?
  - Which institutions (repricing, prominence, reviews) improve welfare?

## Model: market and timing (quick)

- Two firms,  $A$  and  $B$ , know their product qualities (one is better by  $\Delta > 0$ ).
- Consumers arrive (Poisson), observe  $(p_A, p_B)$  and past actions (not payoffs), get private signal with precision  $q \in (\frac{1}{2}, 1)$ , may pay search/switch cost  $\kappa$ .
- Public belief  $\eta(t) = \text{prob. } A \text{ is better}$ , updated from actions (BHW-style).
- Baseline: prices fixed at  $t = 0$ ; later we allow Calvo resets (Poisson opportunities).

## Consumer decision: a single threshold (posterior space)

Start at  $A$ , observe signal  $\Rightarrow$  posterior  $x \in (0, 1)$  that  $A$  is high.

Buy  $A$  without checking iff

$$x \geq x^*(p_A - p_B, \kappa) = \frac{1}{2} + \frac{p_A - p_B - \kappa}{2\Delta}.$$

Otherwise pay  $\kappa$  to check and buy the higher expected surplus.

**Notes:**  $x^*$  increases in  $(p_A - p_B)$ , decreases in  $\kappa$ ; symmetric when starting at  $B$ .

## Cascade bands and absorption

Define posteriors after  $s = A$  and  $s = B$ :

$$\eta_A(\eta) = \frac{q\eta}{q\eta + (1-q)(1-\eta)}, \quad \eta_B(\eta) = \frac{(1-q)\eta}{(1-q)\eta + q(1-\eta)}.$$

Up-absorbing band: smallest  $\eta$  solving  $\eta_B(\eta) = x^*(p_A - p_B, \kappa)$  gives  $\bar{\eta}$ .

Down-absorbing band: largest  $\eta$  solving  $\eta_A(\eta) = 1 - x^*(p_B - p_A, \kappa)$  gives  $\underline{\eta}$ .

**Absorption:** starting from any interior  $\eta_0$ , belief hits  $[0, \underline{\eta}] \cup [\bar{\eta}, 1]$  a.s.; arrival rate  $\lambda$  only time-changes the clock.

## Belief dynamics: sample paths

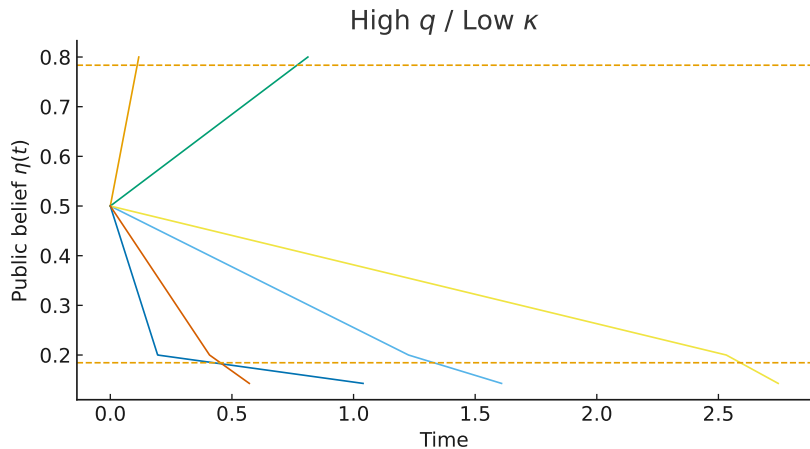

Dashed lines: absorbing bands  $[0, \underline{\eta}]$  and  $[\bar{\eta}, 1]$ .

## Belief dynamics: sample paths

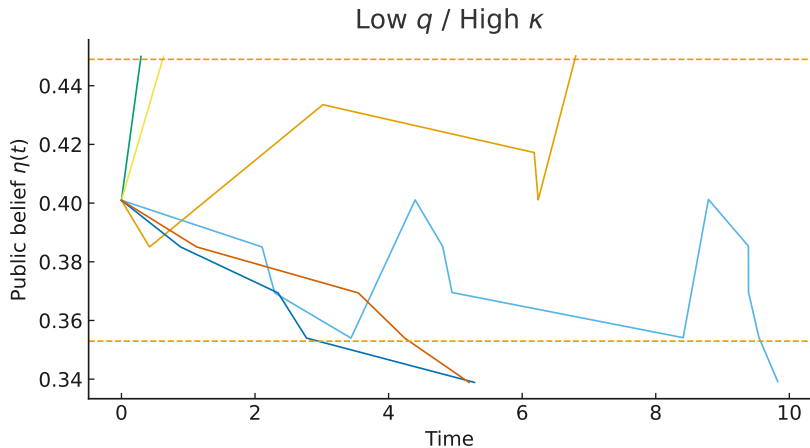

Dashed lines: absorbing bands  $[0, \underline{\eta}]$  and  $[\bar{\eta}, 1]$ .



# Absorption times and wrong cascades

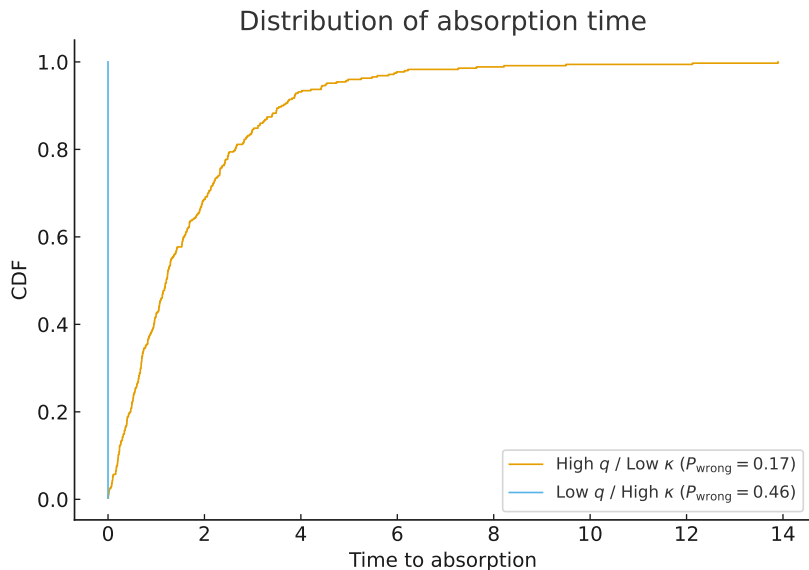

CDF of time to absorption (arrival time). Legend shows  $P_{\text{wrong}}$ .

## Static price competition: existence (discontinuous game)

**Game:** firms choose  $p_A, p_B \in [0, \bar{p}]$  at  $t = 0$ ; payoffs  $\pi_i = p_i \cdot \mathbb{E}[N_i]$ .

**Discontinuities:** knife-edges when posteriors hit  $x^*$ ; measure-zero under mixing.

**Result:** a (symmetric) mixed BNE exists (Reny-style).

- Payoffs bounded; upper semicontinuous in prices.
- Better-reply secure with atomless opponent mixing  $\Rightarrow$  equilibrium.

## Structure & dispersion

- In symmetric mixed equilibrium: supports are *connected, overlapping*, and atomless.
- Dispersion (support width) shrinks with  $q$  (more informative actions) and expands with  $\kappa$  (less checking).
- Mean price co-moves with dispersion (competition tighter when learning is informative).

# Comparative statics & welfare: what moves outcomes?

- **Learning side:**  $q \uparrow$  and  $\kappa \downarrow \Rightarrow$  faster convergence and fewer wrong cascades.
- **Pricing side:** effective demand steepens as actions become more informative.
- **Welfare accounting:** prices are transfers; welfare = accuracy gains — search costs.

## Planner benchmark & policy

- Planner internalizes information externality from checking  $\Rightarrow$  socially optimal cutoff.
- **Pigouvian search subsidy** implements planner's cutoff (state-contingent).
- Prominence and reviews act via informativeness rather than price regulation.

## Extension I: Calvo price resets

- Each firm gets Poisson reset opportunities (hazard  $\alpha$ ); between resets, prices stick.
- Frequent resets shorten stale-price spells, re-start informative sampling.
- **Result:** stationary Markov reset equilibrium exists; dispersion and mean prices fall in  $\alpha$ ; with sufficiently informative signals, wrong-cascade risk falls.

# Calvo dynamics: time series

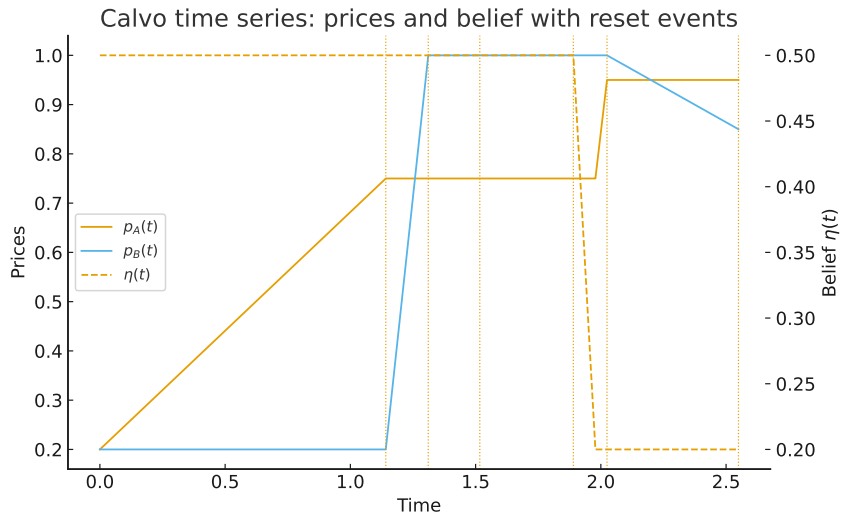

Legend at center-left:  $\eta(t)$ ,  $p_A(t)$ ,  $p_B(t)$ .

## Extension II: Prominence (default ordering)

- First-visit probability  $\phi$ : biasing  $\phi \neq \frac{1}{2}$  softens competition for the prominent firm.
- **Prices:** dispersion width and mean prices increase in  $|\phi - \frac{1}{2}|$ .
- **Welfare:** ex-ante under symmetric prior, neutral prominence  $\phi = \frac{1}{2}$  minimizes wrong-cascade risk and maximizes welfare.



## Extension III: Noisy outcomes (reviews)

- With probability  $\mu$ , a public review  $R_t \in \{+, -\}$  appears; accuracy  $r > 1/2$ .
- Blackwell improvement: absorbing bands shrink; wrong-cascade probability falls.
- Prices: dispersion width and mean fall in review informativeness  $(\mu, r)$ ; in the limit, approach common-knowledge benchmark.

# Takeaways

- Embedding social learning into duopoly pricing yields *endogenous* price dispersion.
- Dispersion and mean prices are disciplined by informativeness:  $q \uparrow$  or  $\kappa \downarrow \Rightarrow$  tighter competition.
- Calvo repricing, neutral prominence, and informative reviews are *information-centric* tools that improve outcomes without direct price controls.

Thank you!

`georgy.lukyanov@tse-fr.eu`

Replication package available on request.

## Absorption & arrival rate

Belief hits  $[0, \underline{\eta}] \cup [\bar{\eta}, 1]$  a.s. in finite *arrival* time.

Poisson arrival rate  $\lambda$  only time-changes:  $\tau_\lambda \stackrel{d}{=} \tau_1/\lambda$ ; absorption probabilities are invariant.

## Existence: discontinuities & security

Knife-edges (posteriors hitting  $x^*$ ) are measure-zero under atomless mixing  $\Rightarrow$  upper semicontinuity.

Better-reply security  $\Rightarrow$  mixed equilibrium (Reny, 1999).

# Notation

$q$  signal precision;  $\kappa$  search cost;  $\eta(t)$  public belief;  $p_A, p_B$  posted prices;  
 $x^*(p_A - p_B, \kappa) = \frac{1}{2} + \frac{p_A - p_B - \kappa}{2\Delta}$ ; absorbing bands  $(\underline{\eta}, \bar{\eta})$ .
